# Supplementary material for: Outbreak diversity in epidemic waves propagating through distinct geographical scales
Source: arXiv:2011.03380 ancillary file (2020-11-14)
Supplement: Supplementary file 1 [file suplementar.pdf]

# Supplementary Material: Outbreak diversity in epidemic waves propagating through distinct geographical scales

Guilherme S. Costa [1] Wesley Cota [1] and Silvio C. Ferreira [1,2]

[1] *Departamento de Física, Universidade Federal de Viçosa, 36570-900 Viçosa, Minas Gerais, Brazil*

[2] *National Institute of Science and Technology for Complex Systems, 22290-180, Rio de Janeiro, Brazil*

We present supplementary figures, video and dataset descriptions.

## I. SUPPLEMENTARY FIGURES

In this section we present figures mentioned in the main text for complementary information and different parameter sets. Reader should consult to the parts of main text where they are cited for the discussion.

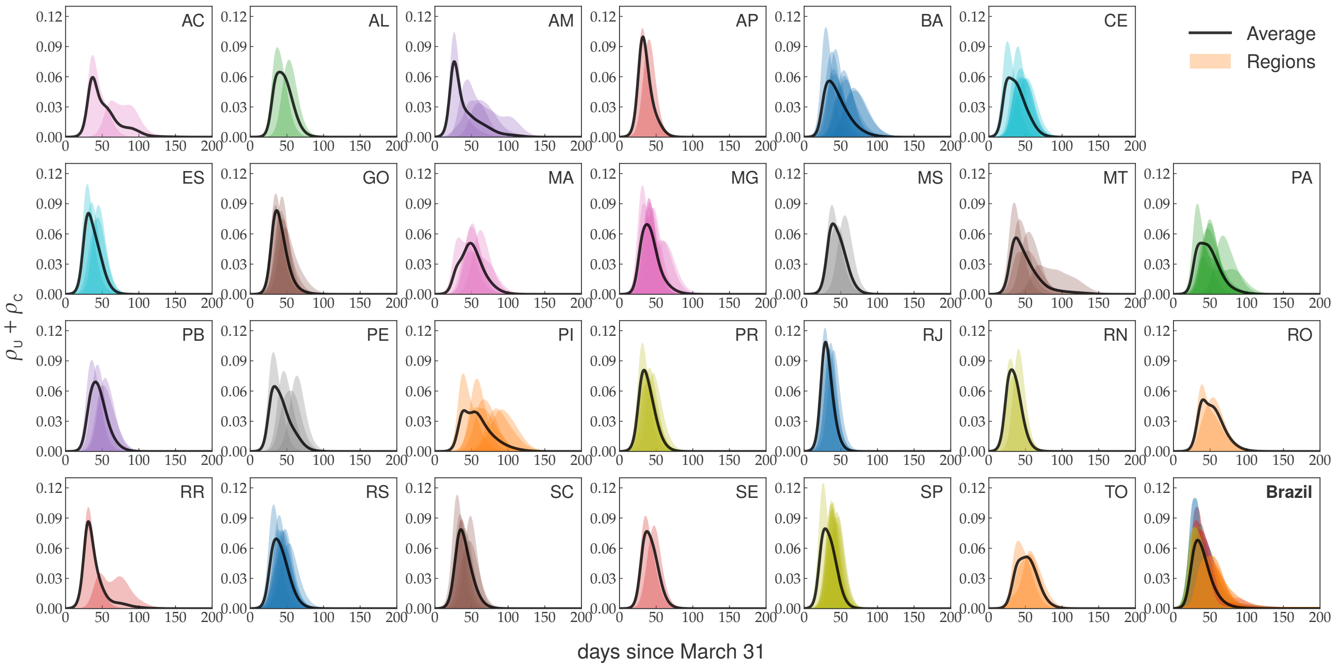


FIG. S1. Epidemic prevalence of symptomatic individuals for all intermediate regions of Brazil grouped by federative state without mitigation obtained with parameters $(M, K) = (0, 0)$. The shaded plots represent the intermediate regions while the thick lines averages within each state. The bottom right corner plot represents an average over the whole country and shaded plots represent federative states.

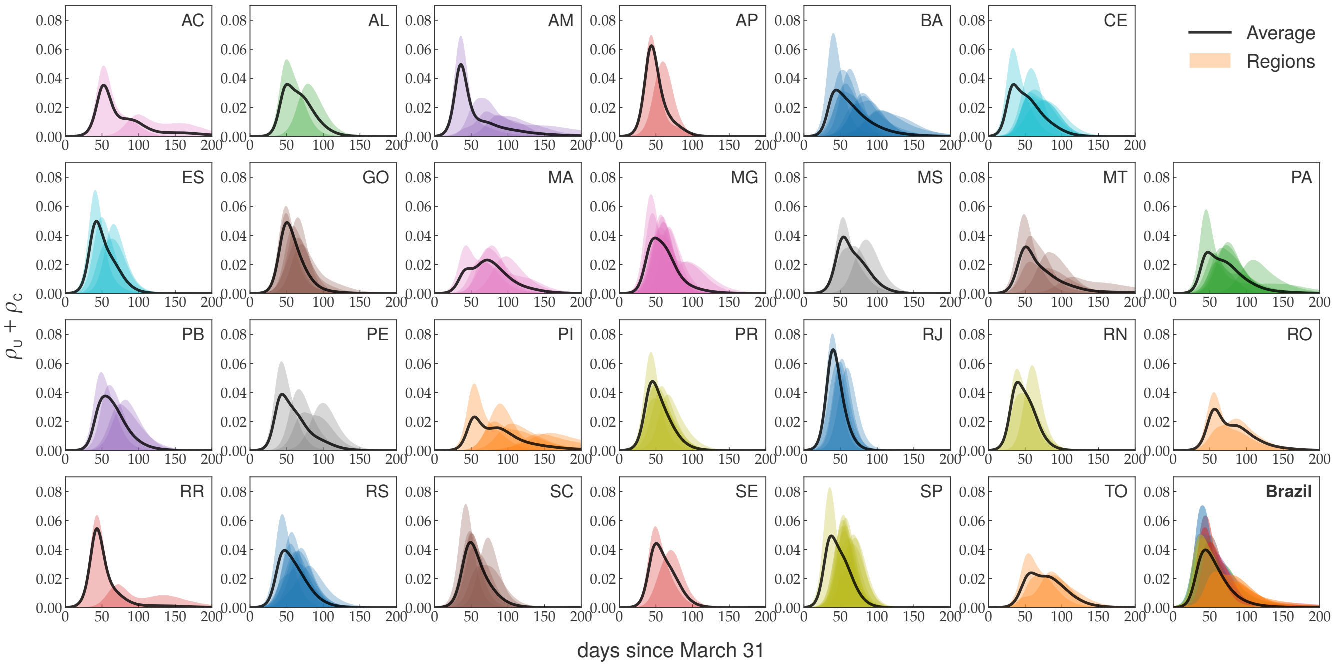


FIG. S2. Epidemic prevalence of symptomatic individuals for all intermediate regions of Brazil grouped by federative state obtained with weak mitigation parameters $(M, K) = (0.4, 0.3)$. The shaded plots represent the intermediate regions while the thick lines averages within each state. The bottom right corner plot represents an average over the whole country and shaded plots represent federative states.

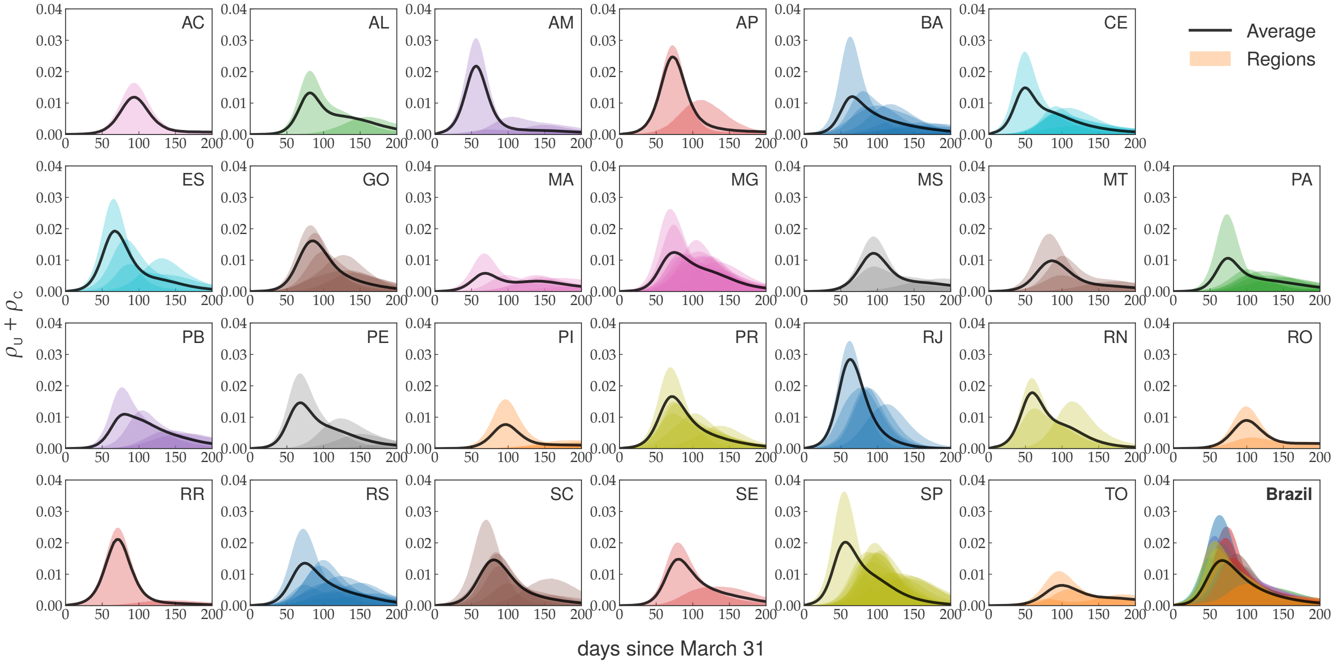


FIG. S3. Epidemic prevalence of symptomatic individuals for all intermediate regions of Brazil grouped by federative state obtained with moderate mitigation parameters $(M, K) = (0.8, 0.5)$. The shaded plots represent the intermediate regions while the thick lines averages within each state. The bottom right corner plot represents an average over the whole country and shaded plots represent federative states.

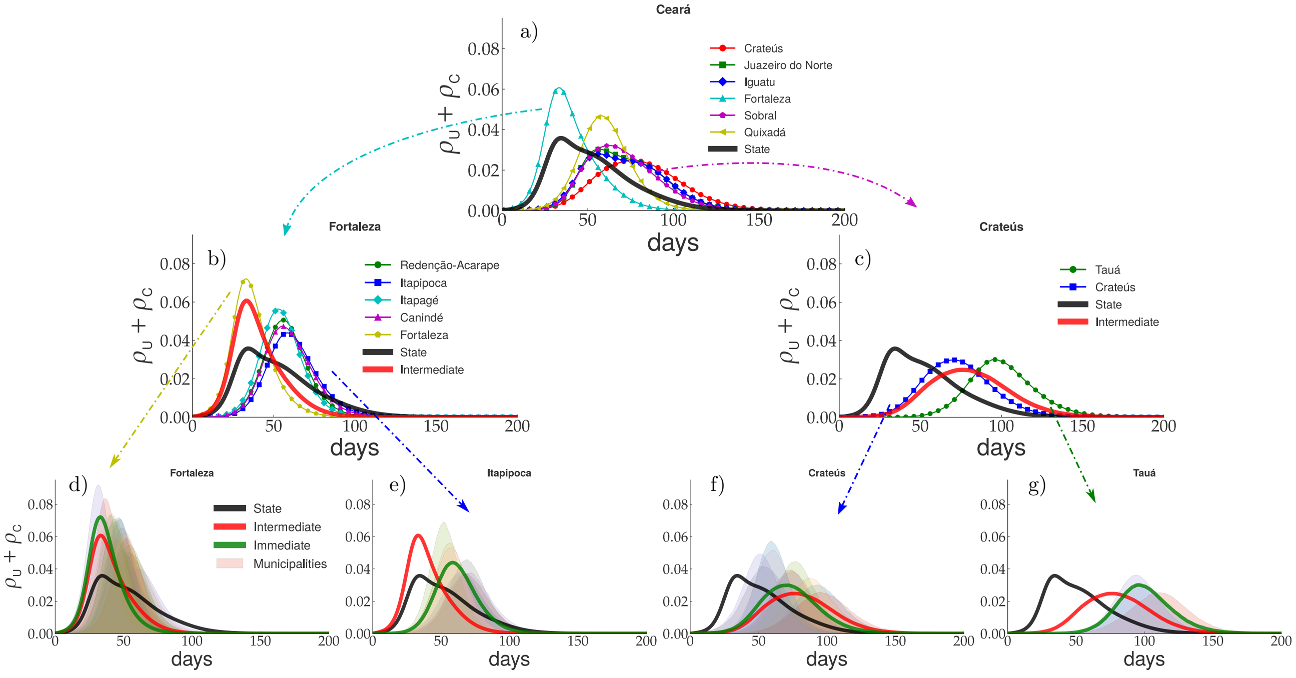


FIG. S4. Multi-scale analysis of the epidemic prevalence of symptomatic individuals for the CE state at several scales of geographical organization considering a weak mitigation with parameters $(M, K) = (0.4, 0.3)$. Epidemic curves averaged with geographical resolution increasing from top to bottom are compared with lower resolution averages: a) intermediate regions, b,c) immediate regions, d-g) municipalities. The curves presenting the earliest and latest maxima are chosen as representative within each panel. Arrows indicate curves selected for zooming. Day 0 represents 31 March 2020.

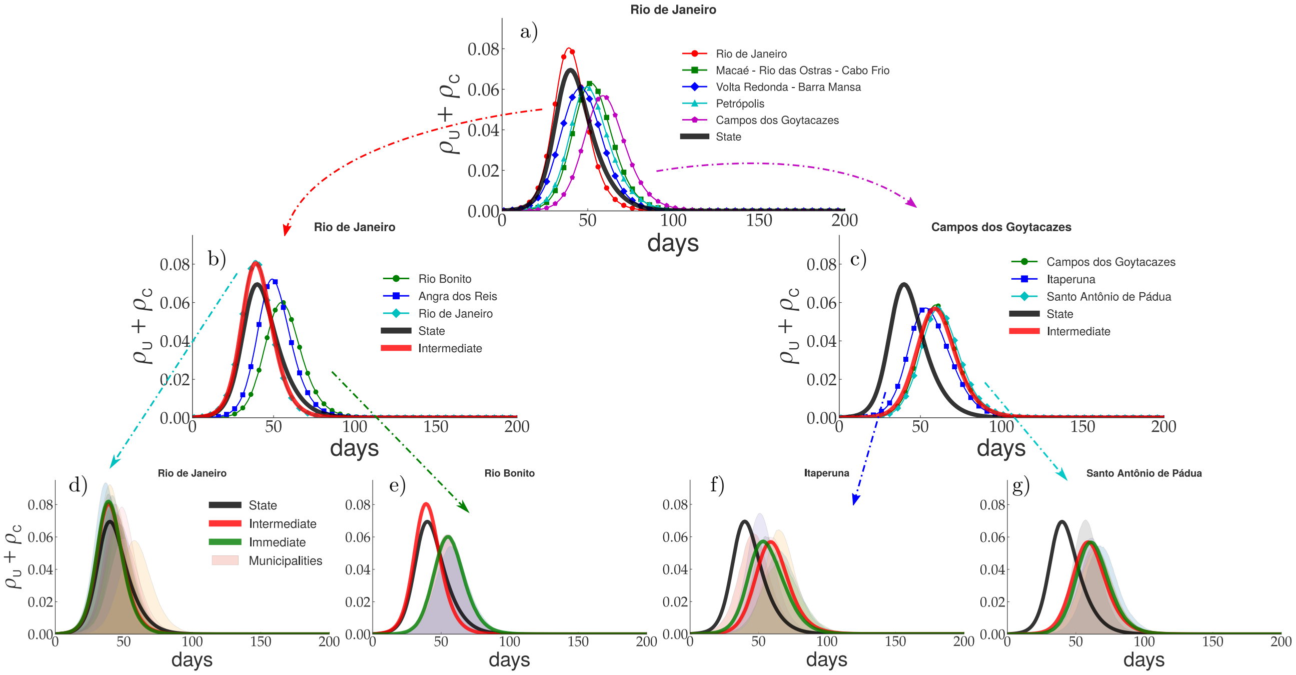


FIG. S5. Multi-scale analysis of the epidemic prevalence of symptomatic individuals for the RJ state at several scales of geographical organization considering a weak mitigation with parameters $(M, K) = (0.4, 0.3)$. Epidemic curves averaged with geographical resolution increasing from top to bottom are compared with lower resolution averages: a) intermediate regions, b,c) immediate regions, d-g) municipalities. The curves presenting the earliest and latest maxima are chosen as representative within each panel. Arrows indicate curves selected for zooming. Day 0 represents 31 March 2020.

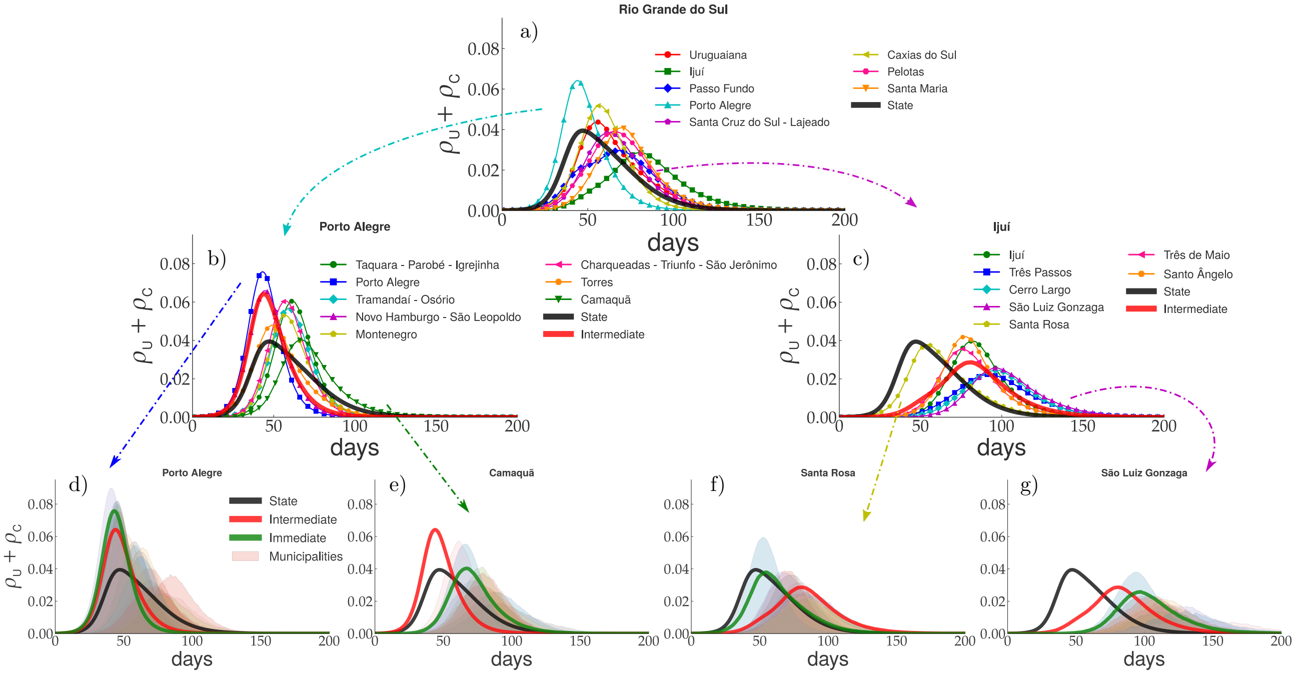


FIG. S6. Multi-scale analysis of the epidemic prevalence of symptomatic individuals for the RS state at several scales of geographical organization considering a weak mitigation with parameters $(M, K) = (0.4, 0.3)$. Epidemic curves averaged with geographical resolution increasing from top to bottom are compared with lower resolution averages: a) intermediate regions, b,c) immediate regions, d-g) municipalities. The curves presenting the earliest and latest maxima are chosen as representative within each panel. Arrows indicate curves selected for zooming. Day 0 represents 31 March 2020.

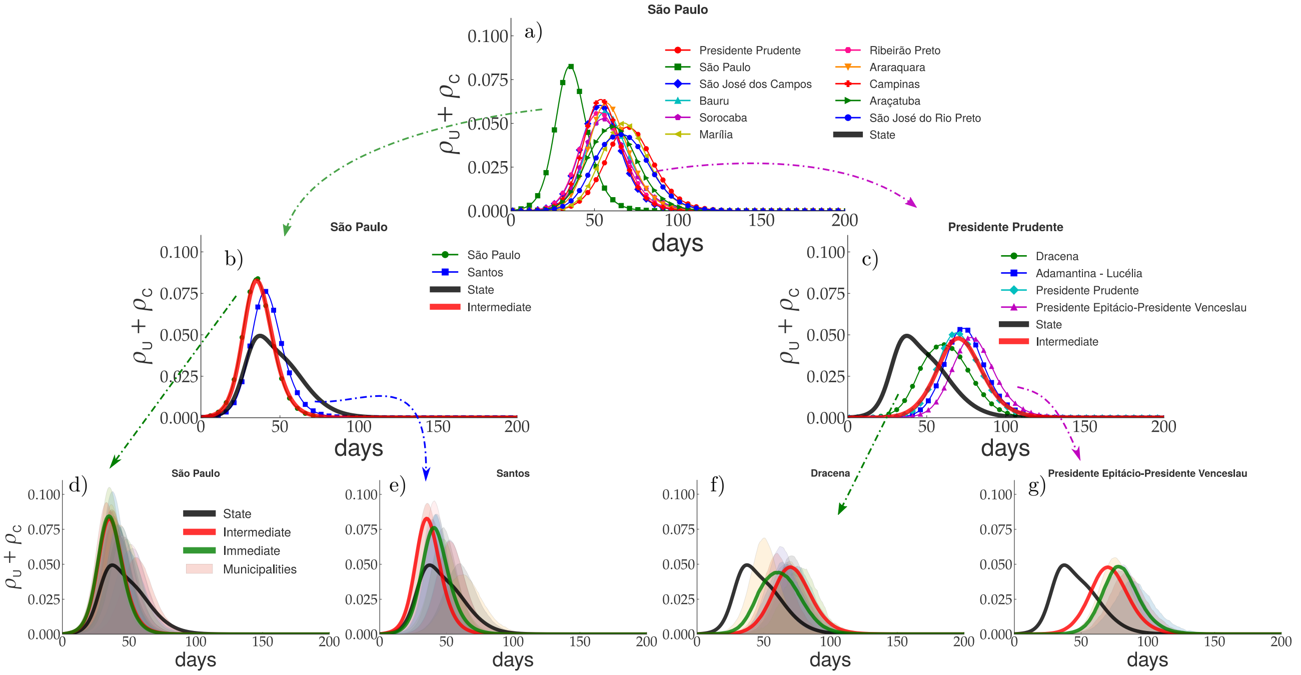


FIG. S7. Multi-scale analysis of the epidemic prevalence of symptomatic individuals for the SP state at several scales of geographical organization considering a weak mitigation with parameters $(M, K) = (0.4, 0.3)$. Epidemic curves averaged with geographical resolution increasing from top to bottom are compared with lower resolution averages: a) intermediate regions, b,c) immediate regions, d-g) municipalities. The curves presenting the earliest and latest maxima are chosen as representative within each panel. Arrows indicate curves selected for zooming. Day 0 represents 31 March 2020.

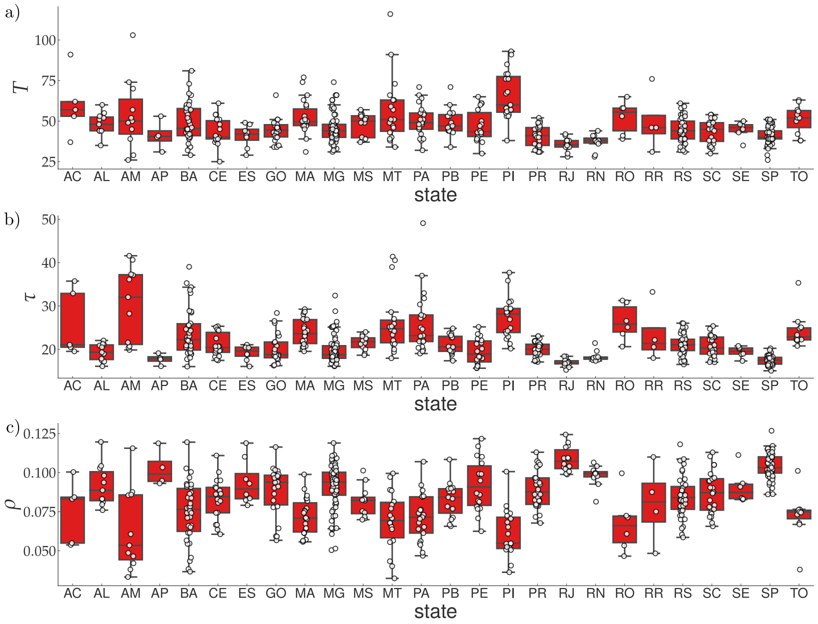


FIG. S8. Box plots for the peak a) time $T$, b) width $\tau$, and c) prevalence $\rho$ averaged over immediate regions for the 26 federation states without mitigation with parameters $(M, K) = (0, 0)$. Circles are data for different regions. As usual, boxes yield median, lower and upper quartiles while points outside whiskers are outliers.

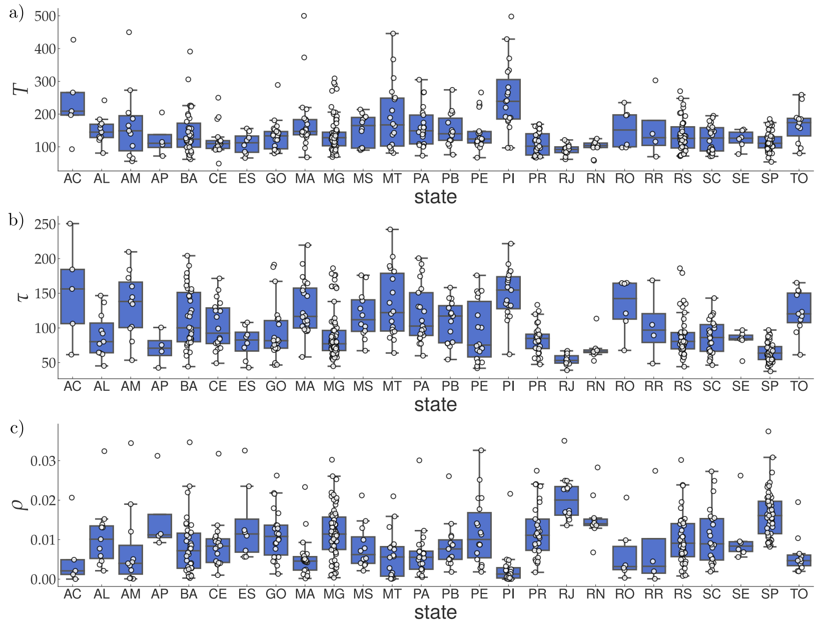


FIG. S9. Box plots for the peak a) time $T$, b) width $\tau$, and c) prevalence $\rho$ averaged over immediate regions for the 26 federation states with moderate mitigation using parameters $(M, K) = (0.8, 0.5)$. Circles are data for different regions. As usual, boxes yield median, lower and upper quartiles while points outside whiskers are outliers.

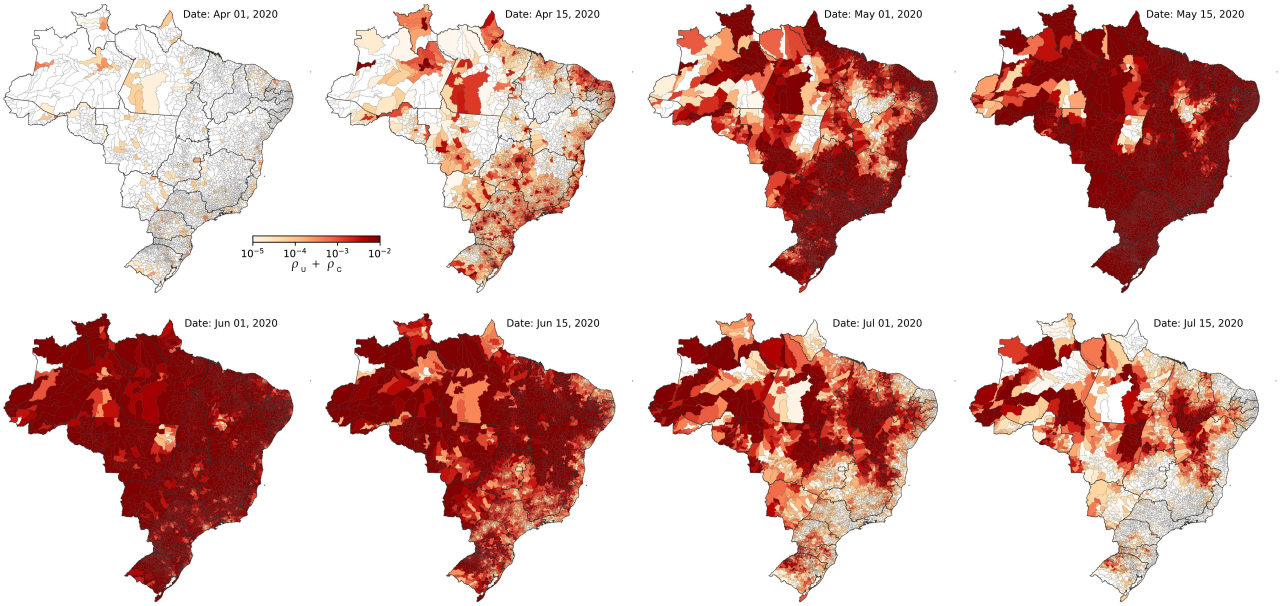


FIG. S10. Color maps with the epidemic prevalence of symptomatic cases (U and C) on Brazil for simulations without mitigation with parameters $(M, K) = (0, 0)$. Dates of the simulations are shown in the upper right corner for all frames. The darker colors represent higher prevalences in a logarithm scale.

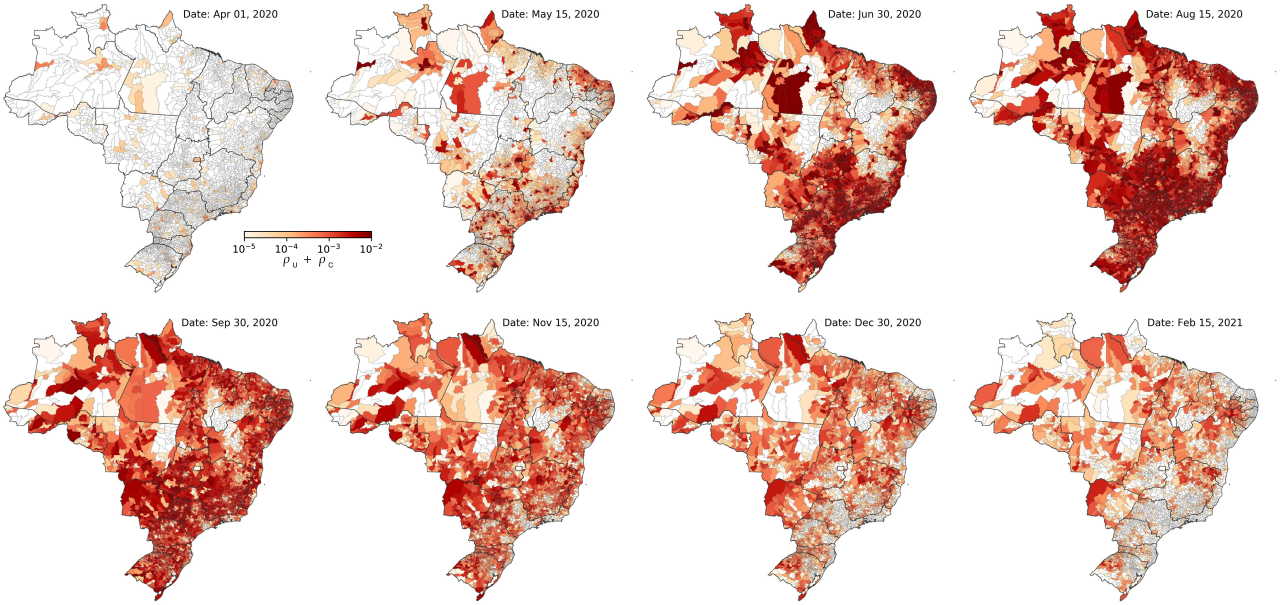


FIG. S11. Color maps with prevalence of symptomatic cases (U and C) on Brazil for a moderate mitigation simulation with parameters $(M, K) = (0.8, 0.5)$. Dates of the simulations are shown in the upper right corner for all frames. The darker colors represent higher prevalences in a logarithm scale.

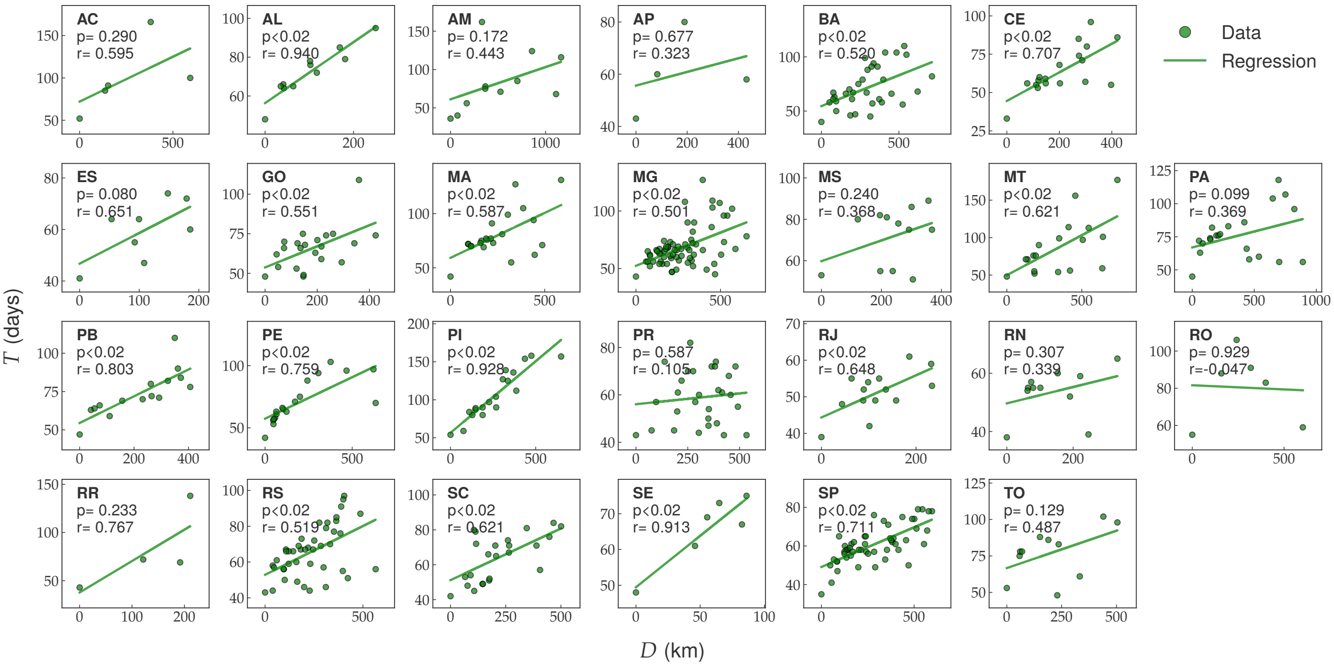


FIG. S12. Scatter plots of days for epidemic peak versus distance from capital city for each federative state of Brazil considering a weak mitigation scenario with parameters $(M, K) = (0.4, 0.3)$. Full lines represent linear regressions o the data. Both $p$-values and Pearson coefficients obtained in the statistical analyses of linear correlations are shown in each panel.

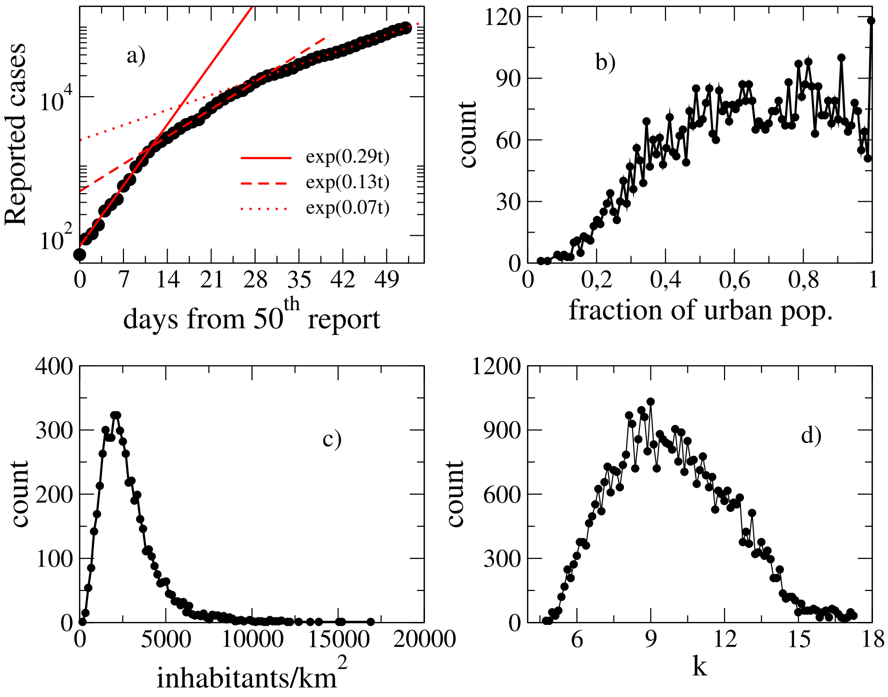


FIG. S13. a) Number of cases of COVID-19 reported in Brazil (Data source: [1]). The day zero correspond to the 50th confirmed case. Histograms for the b) fraction of urban population, c) urban population density, and d) number of contacts $k_i$ in different municipalities; the last one was estimated using the model presented in the main paper.

## II. SUPPLEMENTARY VIDEOS AND DATA DESCRIPTION

Video S1. Daily evolution of the prevalence of symptomatic individuals on Brazilian municipalities for simulations without mitigation with parameters $(M, K) = (0, 0)$. Dates of the simulation are shown in the upper right corner for all frames. The darker colors represent higher prevalences in a logarithm scale.

Video S2. Daily evolution of the prevalence of symptomatic individuals on Brazilian municipalities for simulations using weak mitigation with parameters $(M, K) = (0.4, 0.3)$. Dates of the simulation are shown in the upper right corner for all frames. The darker colors represent higher prevalences in a logarithm scale.

Video S3. Daily evolution of the prevalence of symptomatic individuals on Brazilian municipalities for simulations using moderate mitigation with parameters $(M, K) = (0.8, 0.5)$. Dates of the simulation are shown in the upper right corner for all frames. The darker colors represent higher prevalences in a logarithm scale.

**Confirmed cases used as seeds.** In the file `seeds.csv` of this supplemental material yield the number of confirmed cases for all municipalities in Brazil on 24 March, 31 March, and 04 April 2020 used to build the seeds for the initial condition. They were extracted from Ref. [1].

[1] W. Cota, "Monitoring the number of COVID-19 cases and deaths in Brazil at municipal and federative units level," SciELOPreprints:362 (2020), 10.1590/scielopreprints.362.
